# Supplementary material for: Learning Gradient Fields for Molecular Conformation Generation
Source: arXiv:2105.03902 source file (2021-06-08)
Supplement: Supplementary file 1 [file cov-mat-suppl-ff.tex]

\begin{tabular}{l | cccc | cccc}
\toprule
\multirow{3}{*}{Method} & 
\multicolumn{4}{c|}{GEOM-QM9} &
\multicolumn{4}{c}{GEOM-Drugs} \\
& \multicolumn{2}{c}{COV$^*$ (\%)} 
& \multicolumn{2}{c|}{MAT (\AA)} 
& \multicolumn{2}{c}{COV$^*$ (\%)} 
& \multicolumn{2}{c}{MAT (\AA)} \\
& Mean & Median & Mean & Median 
& Mean & Median & Mean & Median \\
\midrule
RDKit & 83.26 & 90.78 & 0.3447 & 0.2935 & 60.91 & 65.70 & 1.2026 & 1.1252 \\
CVGAE + FF &  &  &  &  &  &  &  & \\
GraphDG + FF &  &  &  &  &  &  &  & \\
CGCF + FF & 83.20 & 85.56 & 0.3001 & 0.2578 & 92.64 & 98.73 & 0.7765 & 0.7502 \\
\textbf{\method + FF} & \textbf{85.70} & \textbf{90.05} & \textbf{0.2492} & \textbf{0.2419} & \textbf{93.61} & \textbf{98.84} & \textbf{0.7596} & \textbf{0.7428} \\
%\textbf{\methodd + FF} & 83.57 & 86.51 & 0.3016 & 0.2549 & 92.63 & 98.31 & 0.7709 & 0.7520 \\    
\bottomrule
\end{tabular}
